# Supplementary material for: Experimental set-up for thermal measurements at the nanoscale using an SThM probe with niobium nitride thermometer
Source: arXiv:2403.05405 source file (2024-04-30)
Supplement: Supplementary file 1 [file SM_Swamisub2final.pdf]

# Supplementary Materials (SM)

For ”Experimental set-up for thermal measurements at the nanoscale using an SThM probe with niobium nitride thermometer” by R. Swami,[1, 2] G. Julié,[1, 2] S. Le-Denmat,[1, 2] G. Pernot,[3] D. Singhal,[1, 2] J. Paterson,[1, 2] J. Maire,[1, 2] J.F. Motte,[1, 2] N. Paillet,[1, 2] H. Guillou,[1, 2] S. Gomès,[4] and O. Bourgeois[1, 2]

[1)]*Institut Néel, CNRS, 25 avenue des Martyrs, 38042 Grenoble, France*
[2)]*Université Grenoble Alpes, Institut Néel, 38042 Grenoble, France*
[3)]*Université de Lorraine, CNRS, LEMTA, 54000 Nancy, France*
[4)]*CETHIL, CNRS, 9 Rue de la Physique, 69621 Villeurbanne, France*

- SI1-Thermal conductance of the probe-sapphire contact
- SI2- Thermal contact resistances found in literature and measured values in this work
- SI3- Thermal resistance of the mechanical contact $R_c$ as a function of the force applied

## SI1-Thermal conductance of the probe-sapphire contact

Considering the tip contact radius ($b_c$) measured by SEM at 125 nm and using Eq. 9 (in the manuscript), we can estimate that $G_{sample}$ is 6.15x$10^{-6}$ W $K^{-1}$ and $G_c$ is 7.5x$10^{-8}$ W.$K^{-1}$ (**$R_c$=13.5 K µ$W^{-1}$**), which corresponds with a thermal boundary resistance (TBR) of 6.6x$10^{-7}$ K $m^2$ $W^{-1}$. However, the mechanical contact radius could be less than 125 nm. Using the out-of-contact and in-contact $T_{2\omega}$ results and Eq. 11 (in the manuscript), we estimated the thermal conductance of the sapphire-contact probe and associated TBR for various values of mechanical contact radius below this value of $b_c$ (125 nm). The results are given in Table S1 for $b_c$ values of 100, 50 and 20 nm.

***Table S1: Components of the thermal resistance at the tip and thermal boundary resistance for different contact radii.***

| $b_c$ (nm) | **125** | **Uncertainty[b]** | 100 | 50 | 20 |
|---|---|---|---|---|---|
| $G_{sample}$ (W.$K^{-1}$)[a] | **6.2 x$10^{-6}$** | **± 1.5 x$10^{-6}$** | 4.24 | 1.26 | 0.23 |
| $G_c$ (W.$K^{-1}$) | **7.5x$10^{-8}$** | **± 2 x$10^{-8}$** | 7.5 x$10^{-8}$ | 7.8x$10^{-8}$ | 1.1 x$10^{-7}$ |
| $R_c$ (K.$W^{-1}$) | **13.5 x$10^{6}$** | **± 3.6 x$10^{6}$** | 13 x$10^{6}$ | 13 x$10^{6}$ | 9.3 x$10^{6}$ |
| $R_{tip\ apex}$ (K.$W^{-1}$) | **1.0 x$10^{4}$** | **-** | 1.0 x$10^{4}$ | 1.0 x$10^{4}$ | 1.0 x$10^{4}$ |
| *TBR* (K.$m^2$.$W^{-1}$) | **6.6 x$10^{-7}$** | **2.8 x$10^{-7}$** | 4.2 x$10^{-7}$ | 1.0 x$10^{-8}$ | 1.2 x$10^{-8}$ |

[a] Values calculated using a value of the thermal conductivity elsewhere measured of 34 W $m^{-1}$ $K^{-1}$ [s1] and the phonon average mean free path for sapphire of 130 nm at 300 K as in reference [s2].

[b] Uncertainty values in Table S1 refer to a $b_c$ value at 125±10 nm and a noise-to-signal ratio of 2 µVolt (noise) /6 mV (signal), which corresponds to a relative uncertainty on $T_{2\omega}$ and $G_{probe}$ of $\Delta T_{2\omega}/T_{2\omega} = \Delta G_{probe}/G_{probe}$ =3 x$10^{-4}$.

## SI2- Thermal contact resistances found in literature and measured values in this work

Table S2 gives the values of thermal contact resistance ($R_c$) found in literature for two types of probes (Pd and DS probes) operated in vacuum conditions with different pressures and tip-sample forces. We can observe that our result, $R_c$=13.5 ± 3.6 K µW$^{-1}$ is close to those obtained in vacuum at pressures ($P$) lower than 10$^{-3}$ mbar using Pd probes, which have a curvature radius close to the NbN probe.

***Table S2: Comparison of different thermal contact resistances found in literature and measured values in this work.***

| $R_C$ | Probe temperature/heating regime | Probe type | Sample surface | Vacuum pressure | Thermal contact radius/force | Reference |
|---|---|---|---|---|---|---|
| K µW$^{-1}$ | K | | Material | mBar | nm/nN | |
| 2.3±0.4 | 338/DC | Pd probe | Si[b] | 0.28 | 50/75 | [s3] |
| 1.4±0.1 | | | Ge[b] | | 50/75 | |
| 15 | - | Pd probe | ZnO | 1.3x10$^{-3}$ | 50/3 | [s4] |
| 41.6±3.5 | - | Pd probe | $SiO_2$ | <10$^{-4}$ | - | [s5] |
| 9.4±0.2 | 333/3ω-SThM | Pd probe | Si[b] | 10-5 | 100 nm/- | [s6] |
| 6.0±0.2 | 373/3ω-SThM | Pd probe | Au | 10-5 | | |
| 54±1 | 308 | Pd probe | $SiO_2$ | 2x10$^{-6}$ | 23/ minimal indentation set point | [s7] |
| 6±2 | 885 | DS probe | $SiO_2$/$HfO_2$ | 10$^{-5}$ | 14/<10 | [s8] |
| 8.6±0.4 | - | DS probe | $SiO_2$ | <10$^{-4}$ | - | [s5] |
| 2±1 | 318 | SiNx AFM probe with Pt sensor, Cr layer on tip | Si[a] 298 K | 10$^{-9}$ | 5.5/50 | [s9] |
| 1.1 ±0.1 | 318 | | Si[a] 603.15 K | 10$^{-9}$ | | |
| **13.5±3.6** | **5 K above room temperature/ 3ω-SThM** | **$SiN_x$ AFM probe with NbN sensor** | **Sapphire** | **3 10$^{-6}$** | **125/20** | **This work** |

[a] Heated sample [b] Native oxide layer -[c]– data not available

Considering the Pd probe, as expected, Table S2 shows that:

- larger is the pressure $P$ lower $R_c$ is. For $P$ >10$^{-3}$ mbar [s3], heat can be transferred by the water meniscus that can still form at the tip-sample contact at this pressure level, explaining a lower value of $R_c$ in this case.
- larger the applied force is lower the $R_c$ value is [s8].
- ensuring metal at the apex of tip [s9] enables to decrease $R_c$ even at pressure of 10$^{-9}$ mbar.

As for the NbN probe, the metallic sensor of the Pd probe covers a SiN tip. However, the Pd probe is manufactured so that Pd covers the tip apex contrarily to the NbN probe. If the metal at the apex contributes to increasing the amount of heat transferred from the self-heated tip to the sample in the case of the Pd probe, a mechanical wear of the probe (after scanning the surface of a sample for example) can lead to the elimination of the Pd at the tip apex. This could explain why our results are close to those obtained with the Pd probe: $R_c$ values obtained using the two probes correspond to thermal resistances between SiN and the sample material.

## SI3- Thermal resistance of the mechanical contact $R_c$ as a function of the force applied

Figure S1 gives the evolution of the value of $R_c$, calculated using $b_c$=125 nm, as a function of the force applied to the probe over the range [5 - 50 nN]. We assume that $b_c$ does not change significantly with the force increasing. We can observe that increasing the force leads naturally

to an improvement of the mechanical contact, by flattening of the tip apex for instance, but the change in $R_c$ (2.5 K µW$^{-1}$) is not significant compared with the uncertainty of the $R_c$ value estimated at 3.6 K µW$^{-1}$. This demonstrates the good reproducibility of measurements with the NbN probe while it is used with a force lower than 50 nN, which is in the order of magnitude of the forces used in SThM (see Table S2).

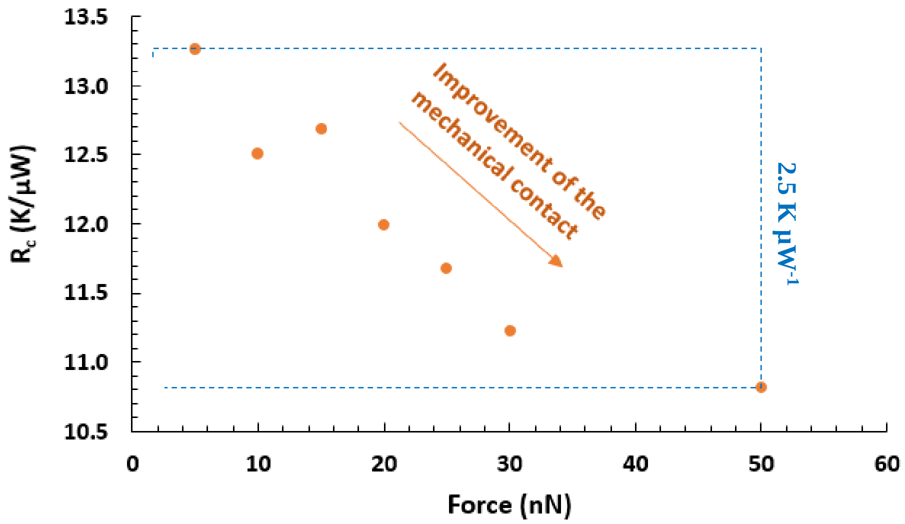


***Figure S1: Variation of the thermal resistance of the mechanical contact $R_c$ as a function of the force applied. The equivalent contact radius $b_c$ is taken to be 120 nm in the estimation of $R_c$.***

## SI4- Details on the 3D COMSOL® thermal modeling of the probe

Post-processing analysis of Comsol® results and 3ω voltage evaluation.
From our 3D Comsol® model, we are able to evaluate the variation of the voltage across the probe as a function of time. An example of this raw voltage signal is given in the next figure for an excitation frequency of 5Hz.

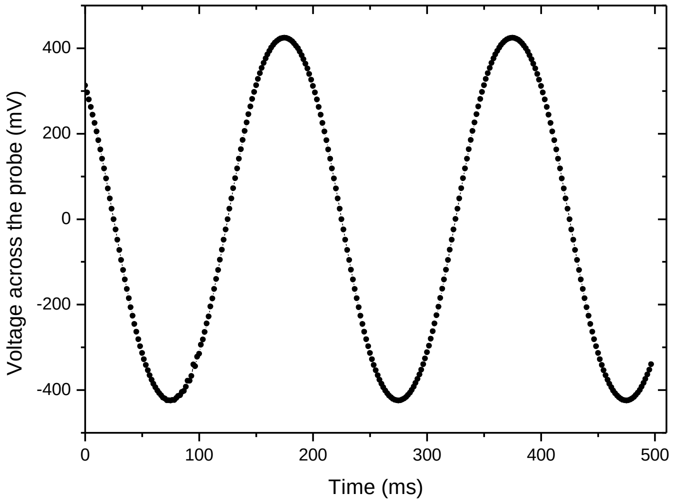


***Figure S2: Raw voltage across the NbN probe calculated using our 3D Comsol Multiphysics model.***

As explained in ref [31] of the main text, a temporal discretization of 120 points per period and a simulation time of 2.5 periods are sufficient to obtained stable values for the amplitude and phase of the signal. This raw signal contains the 1st and 3rd harmonics of the voltage according to the equation:

$$V_0(t) = V_\omega \cdot \cos(\omega t + \varphi_\omega) + V_{3\omega} \cdot \cos(3\omega t + \varphi_{3\omega})$$

where $V_\omega$, $\varphi_\omega$ are respectively the amplitude and phase of the 1st harmonic voltage and $V_{3\omega}$ and $\varphi_{3\omega}$ are the amplitude and phase of the 3rd harmonic voltage.

Using a fitting algorithm with the following function:

$$F(t) = A_1 \cdot \cos(\omega t + \varphi_1) + A_2 \cdot \cos(3\omega t + \varphi_2)$$

where $A_1$, $A_2$, $\varphi_1$ and $\varphi_2$ are the free parameters of fitting algorithm. We obtain the amplitude and phase of the first and third harmonics. The procedure {FEM simulation – post-processing} is repeated for all the frequencies, and rms-$V_{3\omega}$ values given in figure 8-b of the main text are the values of the parameter $A_2$ divided by √(2). The following figure shows the results of the post-processing analysis.

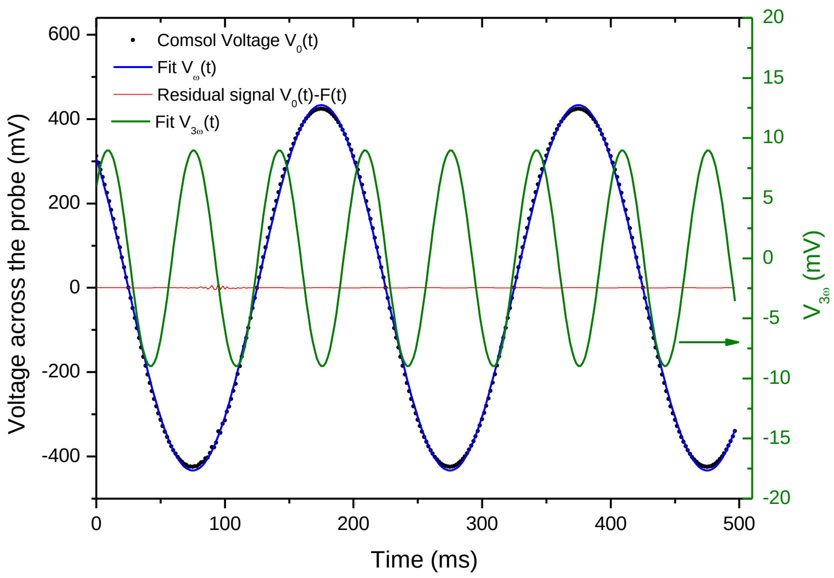


***Figure S3*: Results of the post-processing analysis and evaluation of the 3ω amplitude.**

The blue curve represents the 1st harmonic component of the voltage according to the equation:

$$V_\omega(t) = A_1 \cdot \cos(\omega t + \varphi_1)$$

The green curve represents the 3rd harmonic component of the voltage given by:

$$V_{3\omega}(t) = A_2 \cdot \cos(3\omega t + \varphi_2)$$

and the red curve shows the residual signal:

$$Residual(t) = V_0(t) - F(t) = V_0(t) - [A_1 \cdot \cos(\omega t + \varphi_1) + A_2 \cdot \cos(3\omega t + \varphi_2)]$$

## References


s1. J. Paterson, “Experimental investigation of heat transport in nanomaterials using electrothermal methods,” Thesis Grenoble (2020)

s2. K. M. Hoogeboom-Pot, J. N. Hernandez-Charpak, X. Gu, T. D. Frazer, E. H. Anderson, W. Chao, R. W. Falcone, R. Yang, M. M. Murnane, H. C. Kapteyn, and D. Nardi, “A new regime of nanoscale thermal transport: Collective diffusion increases dissipation efficiency PNAS 112, 4846–4851 (2015)

s3. A. Assy, S. Gomès, “Heat transfer at nanoscale contacts investigated with scanning thermal microscopy”, Appl. Phys. Lett. 2015, 107, 043105.

s4. D. Alikin, K. Zakharchuk, W. Xie, K. Romanyuk, M. Pereira J., B. I.Arias-Serrano, A. Weidenkaff, A. Kholkin, A. V. Kovalevsky, “Quantitative Characterization of Local Thermal Properties in Thermoelectric Ceramics Using “Jumping-Mode” Scanning Thermal Microscopy”, A. Tselev, Small Methods 2023, 7, 14

s5. Z. Umatova, Y. Zhang, R. Rajkumar, P. S. Dobson, J. M. R. Weaver, “Quantification of atomic force microscopy tip and sample thermal contact”, Rev. Sci. Instrum. 2019, 90, 095003.

s6. G. Pernot, A. Metjari, H. Chaynes, M. Weber, M. Isaiev, D. Lacroix, “Frequency domain analysis of 3ω-scanning thermal microscope probe—Application to tip/surface thermal interface measurements in vacuum environment”, J. Appl. Phys. 2021, 129, 5

s7. S. Gonzalez-Munoz, K. Agarwal, E. G. Castanon, Z. R. Kudrynskyi, Z.D. Kovalyuk, J. Spièce, O. Kazakova, A. Patanè, O. V. Kolosov, “Direct Measurements of Anisotropic Thermal Transport in γ-InSe Nanolayers via Cross-Sectional Scanning Thermal Microscopy”, Adv. Mater. Interfaces 2023, 10, 2300081.

s8. Hinz, M.; Marti, O.; Gotsmann, B.; Lantz, M. A.; Dürig, U. “High resolution vacuum scanning thermal microscopy of $HfO_2$ and $SiO_2$”, Appl. Phys. Lett. 2008, 92, 043122.

s9. A. Reihani, S. Yan, Y. Luan, R. Mittapally, E. Meyhofer, P. Reddy, “Quantifying the temperature of heated microdevices using scanning thermal probes”, Appl. Phys. Lett. 2021, 118, 163102.
